# Supplementary material for: Multi-treatment Effect Estimation from Biomedical Data
Source: arXiv:2112.07574 source file (2023-01-05)
Supplement: Supplementary file 1 [file 9-appendix.tex]

% \section{Extra Details on the Architecture}\label{extra-details}

% \begin{figure}[h]
%     \centering
%     \includegraphics[scale=0.5]{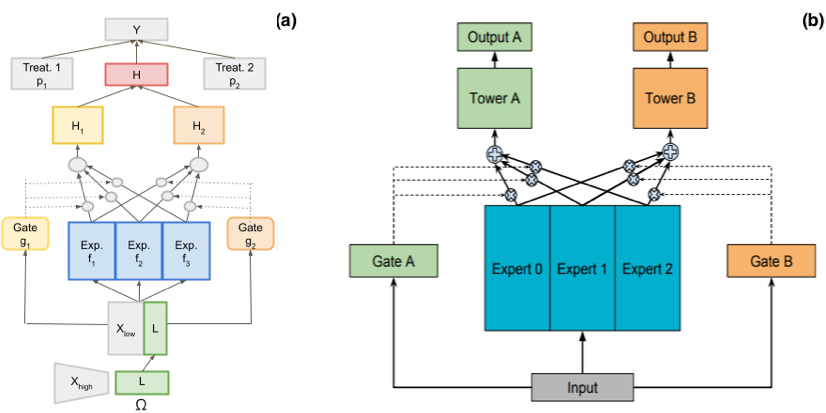}
%     \caption{(a) M3E2 architecture testing architecture. Shows the testing architecture, where the propensity score prediction is not required. (b) The Original MMoE architecture (Figure from \cite{ma2018modeling})}
%     \label{sup1}
% \end{figure}

% Figure \ref{sup1}.a shows the testing architecture. The main difference is that we do not need to use the predicted propensity score for the testing phase. Instead, we use the observed assigned treatments. 

% For comparison, Figure \ref{sup1}.b shows the original MMoE architecture, as proposed by \citet{ma2018modeling}. While the backbone is very similar, our M3E2 architecture has an extra layer with the autoencoder, and the top layers are also different. M3E2 top layer modifies the architecture for the outcome model, which estimates the treatment effect.

\section{Datasets}\label{datasets}

Here we will present a broader description of the datasets adopted to validate our proposed architecture, M3E2. The main goal of our project is to estimate multiple treatment effects by adopting a multi-task learning approach. Furthermore, a given sample can be assigned one or more treatments. First, Table \ref{settings} shows all architectures considered.

\begin{table}[!h]
    \centering
    \caption{Datasets settings explored. Example: Setting \textbf{a} indicates a study on the sample size effect on the GWAS dataset. We compared the models’ MAE with
$2000 \times 4000 \times 6000$ samples, with 5 treatments and 995 covariates.}
    \begin{tabular}{c|c|c|c|c}
    \hline 
        Setting    &  Data & Sample Size & Number of Treatments  & Number of Covariates \\ \hline
        a    &  GWAS & 2000, 4000, 6000 & 5 & 995\\
        b    &  GWAS & 6000 & 5 &100, 500, 1000\\
        c    &  GWAS & 6000& 3, 6, 9& 500\\
        d    &  Copula & 2500, 5000, 10000& 4& 10\\
        e    &  Copula & 10000& 4& 5, 25, 125\\ 
        f & IHDP & 747 & 1 & 24 \\\hline
    \end{tabular}
    \label{settings}
\end{table}

\subsection{GWAS}

We follow the same simulation process available in the literature \cite{song2015testing, wang2019blessings, aoki2020parkca}. The covariates and treatments are single-nucleotide polymorphisms (SNPs), and the target, also referred as the outcome of interest, is a clinical trait. The outcome is continuous, and treatments, binary. We set a small number of SNPs to be causal, meaning they affect the outcome of interest. These causal SNPs are the treatments we want to estimate the treatment effect for. The dataset generation uses as a base the 1000 Genome Project (TGP), used to calculate the matrix of allele frequency $F_{J, V}$, where $J$ is the number of samples and $V$ the number of SNPs. See below the steps to generate the covariates of the simulated dataset:

\begin{enumerate}
    \item We remove highly correlated SNPs with linkage disequilibrium. 
    \item $S_{L\times V} = PCA(TGP)$: First, we extract $L$ principal components from a PCA fitted to the TGP database. For this project, $L=3$
    \item We append a new column to $S$ such that $S_{3, V}=1$ to be the intercept. 
    \item We created a new matrix, $\Gamma_{J, L}$, to represent the simulated samples:
        \begin{equation}
            \Gamma_{j,d} \sim 0.9 \times Uniform(0,0.5) \forall j\in\{1,...,J\}, d\in\{0,1,2\}. 
        \end{equation}
    and $\Gamma_{j,3} = 0.05$
    \item The matrix of allele frequency is obtained from $F_{J, V} = \Gamma_{J, L} \times S_{L, V}$. 
    \item This matrix is then used to simulate the covariates: 
        \begin{equation}
            X_{J, V} \sim Binomial(1, F_{J, V})
        \end{equation}

\end{enumerate}

After simulating the covariates, we simulate the outcome of interest. 
\begin{enumerate}
    \item We define an array $\tau_v,\forall v\in\{0,...,V\}$. We set $\tau_v \neq 0$ for the SNPs used as a treatment, and  $\tau_v = 0$ otherwise. 
    \item Defining the set treatments as K, if $v \in K$, the treatment effect is simulated as $\tau_v\sim Normal(0,0.5)$. 
    \item To add confounding effect, we group individuals using $kmeans(X)$ and three clusters $c$. These clusters are used as per-group intercept $\gamma_{c_j}$ and to define the error variance $\epsilon\sim Normal(0,\sigma_c)$, where $\sigma_1, \sigma_2, \sigma_3 \sim InvGamma(3, 1)$.
    \item Following a high signal-to-noise ration, the SNP's and the per-group intercept are responsible for 40\% ($v_{gene} = v_{group} = 0.4$) of the variance each, and the error is responsible for 20\% ($v_{noise} = 0.2$) of the variance.
    To re-scale the noise and intercept:
    \begin{equation}
       \gamma_j \leftarrow \left[\frac{sd\{ \sum_v\tau_v X_{v,j}\}_{j=0}^J }{\sqrt{v_{gene}}}\right]\left[ \frac{\sqrt{v_{group}}}{sd\{\gamma_j\}^J_{j=0}} \right]\gamma_j
    \end{equation}
    \begin{equation}
       \epsilon_j \leftarrow \left[\frac{sd\{ \sum_v\tau_v X_{v,j}\}_{j=0}^J }{\sqrt{v_{gene}}}\right]\left[ \frac{\sqrt{v_{noise}}}{sd\{\epsilon_j\}^J_{j=0}} \right]\epsilon_j
    \end{equation}
    \item Finally, the outcomes are generated as: 
    \begin{equation}
        Y = \sum_v\tau_v X_{v,j} + \gamma_{c_j} + \epsilon_j
    \end{equation}
\end{enumerate}

\subsection{Copula}

Copula dataset was proposed by \citet{zheng2021copula}. We adopted the setting where the outcome is a non-linear function of the treatments. The target adopted can be either continuous or binary, and in our experiments, we used the continuous $Y$. See below how to simulate this dataset:

\begin{enumerate}
    \item Generate $u_{n,s} \sim Normal(0,1)$, where $n$ is the sample size and $s$ the number of covariates not associated with the outcome. 
    \item If $s>1$, define the confounding effect $c$ as the first component of $PCA(u)$; else, $c=u$.
    \item To help us to simulate the treatment effect, we define $B=[]$ and $T=[c,...,c]_{n,k}\times B$, meaning $c$ is repeated $k$ times, where $k$ is the number of treatments. Then, $T = Normal(0,\sigma_t) + T$.
    \item To help explain the outcome construction, we define the outcome as the sum of three quantities: $y = y_1 + y_2 + y_3$. 
    \begin{enumerate}
        \item $y_1 \sim Normal(0,\sigma_y)_{n\times1}$, represents random noise. 
        
        \item $y_2 = [c * \gamma]_{n\times1}$, where $\gamma$ represents the proportion of confounding effect in $y$, and $\gamma=0$ means no confounding effect. 
        
        \item $y_3 = 3T_1 - T2 + T_3I_{T_3>0}+0.7*T_3I_{T_3\leq0}-0.06T_4-4T_1^2$, which is the contribution of the treatment effects in $y$.
    \end{enumerate}
\end{enumerate}

The implementation followed closely the code made available by \citet{zheng2021copula} in \url{https://github.com/JiajingZ/CopulaSensitivity}. One of the main changes was we changed the implementation from R to Python, as you can see in our repository \url{HIDDEN_FOR_DOUBLE_BLIND_SUBMISSION.}

\subsection{IHDP}

We adopted the repetitions available in the literature. In particular, we used the datasets available at  \url{https://github.com/AMLab-Amsterdam/}.
